# Supplementary material for: Projecting Flood-Inducing Precipitation with a Bayesian Analogue Model
Source: arXiv:1911.05881 ancillary file (2019-11-14)
Supplement: Supplementary file 1 [file SupplementaryMaterial.pdf]

# Supplement to: Projecting Flood-Inducing Precipitation with a Bayesian Analogue Model

Gregory P. Bopp<sup>1</sup>, Benjamin A. Shaby<sup>1</sup>, Chris E. Forest<sup>2</sup>, Alfonso Mejía<sup>3</sup>

## 1 Simulation Study

To evaluate the proposed method, we conduct two simulation studies. In the first, we use a toy model of dynamics to compare the intensity and occurrence models described in Section 2.1 and 2.2 of the main text to modified versions of each where the analogue priors on  $\gamma_t^{(O)}$  and  $\gamma_t^{(I)}$  are replaced by independence priors. In the second simulation study we evaluate the intensity model under more realistic climate dynamics than in the first simulation study using (a) a mixture of Student-t processes and (b) a single Student-t process when the data are generated from (1) a mixture of Student-t processes, (2) a mixture of Gaussian processes, and (3) a single Student-t process.

---

<sup>1</sup>Department of Statistics, Pennsylvania State University, 326 Thomas Building, University Park, PA 16802, U.S.A. Emails: gxb951@psu.edu, bshaby@psu.edu

<sup>2</sup>Department of Meteorology and Atmospheric Science; Department of Geosciences; Earth and Environmental Systems Institute, Pennsylvania State University, University Park, PA 16802, U.S.A. Email: ceforest@psu.edu

<sup>3</sup>Department of Civil and Environmental Engineering, Pennsylvania State University, University Park, PA 16802, U.S.A.

## 1.1 Analogue Prior Assessment Simulation Study

The goal of this section is to evaluate the efficacy of the analogue prior at borrowing strength across time when estimating the location parameters  $\gamma_t$  both for a binary process (occurrence model) and a continuous process (intensity model). To have a clear assessment of the analogue prior in the continuous and binary outcome cases, we will evaluate the two models separately. Furthermore, for the intensity model, we isolate the effect of the analogue prior by considering a single Student-t process, rather than a mixture of Student-t processes (i.e.  $K = 1$ ).

For each of  $M = 50$  Monte Carlo replicates, data are simulated and fit using the following designs. First we describe elements that are common to both the occurrence and intensity simulations. Observation locations are simulated uniformly over the unit square, where the number of observation locations are set to  $n = 15, 30, 60, 120$  for different designs. In each case, the data are simulated for  $T = 500$  time points. The  $L = 16$  spatial basis functions  $\psi_l(\mathbf{s})$ ,  $l = 1, \dots, L$  are taken to be radial Gaussian density basis functions centered at knots that are evenly spaced on the unit square. The spatial basis coefficients are sampled from  $\beta_t \stackrel{\text{iid}}{\sim} N_L(0, \frac{4}{9}I)$ ,  $t = 1, \dots, T$ . To simulate simple time dependence, for both the occurrence and intensity models, the location parameter is constructed as  $\gamma_t = 2 * \sin(2\pi\omega_t t)$  where the frequency  $\omega_t$  linearly increases from  $1/100$  to  $1/30$  as  $t$  increases from 0 to  $T = 500$ ,  $\omega_t = [30 + (T - t) * (100 - 30)/(T - 1)]^{-1}$ ,  $t = 1, \dots, T$ . The parameters of the Matérn correlation functions of both  $\epsilon_t(\mathbf{s})$  in the intensity model and  $Z_t(\mathbf{s})$  of the occurrence model are simulated according to  $\rho \sim \text{Unif}(0, 1/2)$ , and  $\nu \sim \text{Unif}(1/8, 3/2)$ , respectively. The remaining intensity model parameters are simulated as  $a \sim \text{Uniform}(0, 30)$ ,  $b \sim \text{Gamma}(1, 0.1)$ ,

$\sigma_t^2 \stackrel{indep}{\sim} \text{IG}\left(\frac{a}{2}, \frac{ab}{2}\right)$ ,  $t = 1, \dots, T$ . Finally, at every observation location, the intensity response is simulated as  $Y_t(\mathbf{s}) = \gamma_t + \boldsymbol{\psi}(\mathbf{s})'\boldsymbol{\beta}_t + \sigma_t\epsilon_t(\mathbf{s})$ , the latent Gaussian process of the occurrence model is simulated as  $Z_t(\mathbf{s}) \sim \text{GP}(\gamma_t + \boldsymbol{\psi}(\mathbf{s})'\boldsymbol{\beta}_t, c(h))$ , and the occurrences as  $O_t(\mathbf{s}) = 1\{Z_t(\mathbf{s}) > 0\}$ .

For both models we use imperfect information to identify analogues. The distance matrix used for identifying analogues is calculated based on the Euclidean distance between an auxiliary variable that is constructed from the location parameter plus measurement error:  $x_t = \gamma_t + \delta_t$ , where  $\delta_t \stackrel{iid}{\sim} N(0, 1/5)$ ,  $t = 1, \dots, T$ . For comparison, a non-analogue version of the model is estimated where the priors on the location offset is replaced by  $\gamma_t \stackrel{iid}{\sim} N(0, \sigma_\gamma^2)$ ,  $t = 1, \dots, T$ .

To evaluate the performance of the analogue prior, we compare the two proposed models based on the mean squared error (MSE) of  $\gamma_t$  estimates and  $\boldsymbol{\beta}_t$  estimates. The results of this simulation study for varying number of spatial observation locations are given in Figure 1. In both the occurrence model and the intensity model, the MSE of the  $\gamma_t$  estimates is lower when using the analogue prior than for the independence prior. Improved estimates of  $\gamma_t$  also affect the estimation of  $\boldsymbol{\beta}_t$ , which are also lower when an analogue prior is used for  $\gamma_t$  in the occurrence model and comparable in the intensity model. Interestingly, the marginal benefit of the analogue prior decreases as the number of spatial locations increases. This is reasonable since an informative analogue prior allows borrowing of strength across time in estimating the location offset. When the process is observed at many spatial locations, estimation of the offset term becomes easier, and there is less benefit from borrowing of strength over time.

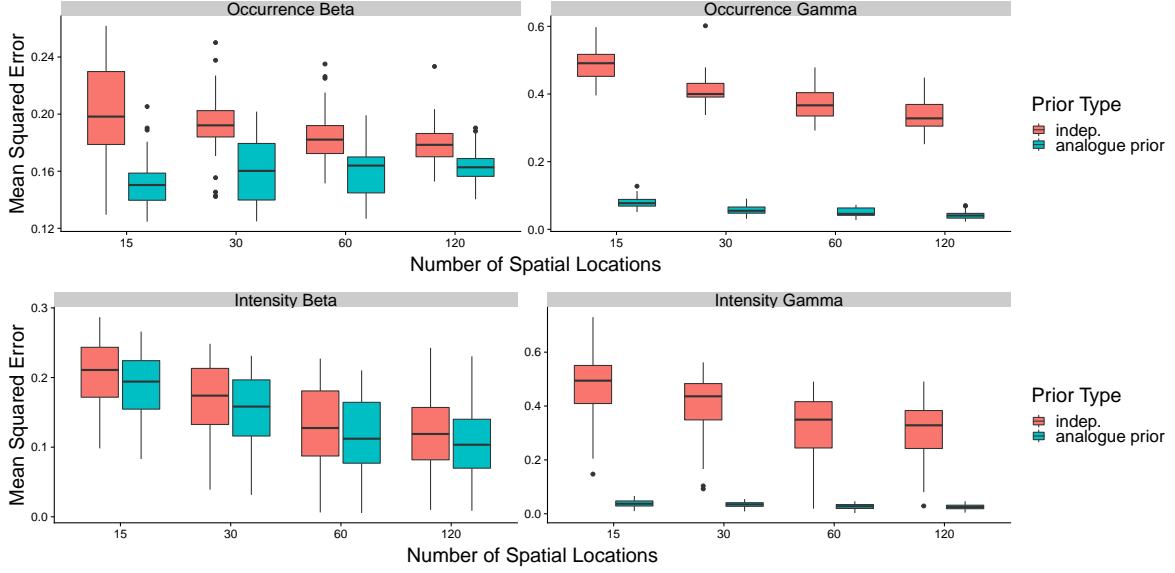

Figure 1: Mean squared error of estimates of  $\gamma_t$  and  $\beta_t$  in the occurrence and intensity models when using an analogue prior on  $\gamma_t$  and an independence prior on  $\gamma_t$  for varying spatial locations.

## 1.2 Climate Control Run Simulation Study

In this section, we evaluate the flexibility of the proposed mixture of Student-t processes as compared to a single Student-t process by fitting both to data simulated under three scenarios: (1) a mixture of Student-t processes, (2) a mixture of Gaussian processes, and (3) a single Student-t process. In the first case, the mixture is the appropriate model for the data; in the second case, the tail dependence of the model is stronger than that present in the data; and in the third case, the mixture is over parameterized.

Data from climate model control runs possess rich temporal dependence with long, stationary time series, providing an interesting test bed for evaluating statistical models under realistic conditions. For this simulation study, we make use of data from the Community Earth System Model (CESM) Large Ensemble project (LENS) climate control run with

Community Atmosphere Model (CAM) 5.2 as its atmospheric component (Kay et al., 2015), which is produced by the National Center for Atmospheric Research (NCAR). Three atmospheric variables are considered, the response, total precipitation rate, and two fields that are used for identifying analogues, geopotential height at 500 hPa pressure and surface temperature. We consider data for three months (April, May, June) from each of 500 years of a climate control run simulated on  $1^\circ \times 1^\circ$  grid cells (357 total) over the northeastern United States and Canada. Climate model control run data should more closely reflect the temporal dependence patterns of precipitation and other atmospheric fields used for identifying analogues in practice than in the first simulation study.

To preserve the temporal structure present in the climate model control run data while varying their spatial dependence structure of the error process according to the three scenarios outlined above, data are simulated as follows: first, for each day of the climate model control run, ridge regression estimates of  $\gamma_t^{(I)}$  and  $\beta_t^{(I)}$ ,  $t = 1, \dots, T$  are found by regressing softplus transformed total precipitation rate on a location offset and radial Gaussian density spatial basis functions centered at 49 knots equally spaced over the observation region, which we denote as  $\check{\gamma}_t$  and  $\check{\beta}_t$ .

Taking the covariates  $\mathbf{u}_t$  in the linear predictor of mixture class membership to be a vector of the first 10 EOF loadings of each of 500 hPa pressure and surface temperature on day  $t$ , and  $\boldsymbol{\alpha}_k \stackrel{\text{iid}}{\sim} N_p(\mathbf{0}, \frac{1}{10}\mathbf{I})$ ,  $k = 1, \dots, K - 1$ , each day is assigned to each of one of  $K = 5$  mixture classes according to probabilities from Equation (1) of the main text, giving roughly balanced classes. Conditional on the mixture class  $\xi_t = k$ , the error process  $\epsilon_t(\mathbf{s})$  is simulated over the 357 spatial locations from a Student-t process or Gaussian process with dependence parameters given in Table 1. Finally, the precipitation process is simulated at each location

Table 1: Dependence parameters for error process  $\epsilon_t(\mathbf{s})$  in climate control run simulation study

| Mixture Class ( $k$ ) | T-Mixture |       |          |         | GP-Mixture   |          |         | Student-t process |       |          |         |
|-----------------------|-----------|-------|----------|---------|--------------|----------|---------|-------------------|-------|----------|---------|
|                       | $a_k$     | $b_k$ | $\rho_k$ | $\nu_k$ | $\sigma_k^2$ | $\rho_k$ | $\nu_k$ | $a_k$             | $b_k$ | $\rho_k$ | $\nu_k$ |
| 1                     | 13        | 20    | 0.15     | 1.2     | 23.6         | 0.15     | 1.2     | 13                | 20    | 0.15     | 1.2     |
| 2                     | 10        | 100   | 0.1      | 1.5     | 125          | 0.1      | 1.5     |                   |       |          |         |
| 3                     | 12        | 35    | 0.15     | 1.3     | 42           | 0.15     | 1.3     |                   |       |          |         |
| 4                     | 10        | 10    | 0.2      | 0.85    | 12.5         | 0.2      | 0.85    |                   |       |          |         |
| 5                     | 13        | 25    | 0.1      | 1.4     | 29.5         | 0.1      | 1.4     |                   |       |          |         |

as  $Y_t(\mathbf{s}_i) = \check{\gamma}_t + \boldsymbol{\psi}(\mathbf{s}_i)' \check{\boldsymbol{\beta}}_t + \epsilon_t(\mathbf{s}_i)$ ,  $t = 1, \dots, T$  for  $i = 1, \dots, n$ . Finally, the distance matrix used for estimating analogues is calculated using lagged vectors ( $r = 3$ ) of the first 10 EOF loadings of each of 500 hPa pressure and surface temperature using the method described in Section 2.3 of the main text. Note that for the Gaussian process mixture, the same simulation settings are used for  $\rho_k$  and  $\nu_k$ , but now the variance parameters for each of the five mixture classes are taken to be the inverse Gamma means from Table 1:  $\sigma_k^2 = \frac{a_k b_k / 2}{a_k / 2 - 1}$ .

The first 30 years are used for training and the remaining 470 years are used for testing. For each simulation design, the intensity model is fit with  $K = 5$  classes and compared to a simpler Student-t process (i.e. the same model with  $K = 1$ ). Out-of-sample posterior predictive draws are made from the model on each holdout day. The models are compared on the basis of how well they capture the tails of the distribution of total precipitation over the field using a tail weighted continuously ranked probability score (TWCPRPS) (Gneiting and Katzfuss, 2014). For a single sample  $y$ , the TWCPRPS is calculated as

$$\text{TWCPRPS}\{\hat{F}, y\} = \int_{-\infty}^{\infty} (\hat{F}(x) - 1\{y \leq x\})^2 w(x) dx, \quad (1)$$

where  $\hat{F}$  refers to the model estimate of the target distribution from which  $y$  is drawn, and

$w(x)$  is a weight function, which for this analysis we take to be  $w(x) = 1\{x \geq q_{0.8}\}$  where  $q_{0.8}$  is the 0.8 quantile of the simulated total precipitation data. In practice, as we do here, the TWCRPS is averaged over a sample  $y_1, \dots, y_T$  as  $\text{TWCRPS} = \sum_{i=1}^T \text{TWCRPS}\{\hat{F}, y_i\}$ . The TWCRPS results are summarized in Figure 2. Lower TWCRPS scores correspond to better correspondence between the empirical and model-based distributions. It is unsurprising that the Student-t mixture outperforms the single Student-t process model when the data are simulated from a mixture of Student-t processes. However, this is also the case when data come from a lighter tailed Gaussian process mixture. In terms of the TWCRPS, the Student-t mixture is also competitive with the single Student-t process when the data are simulated from a single Student-t process. Since scores are estimated based on a holdout set, the simulation results suggest that the proposed Student-t mixture analogue model can accommodate data generated with error processes following both mixtures of Student-t processes and mixtures of Gaussian processes better than a single Student-t process alone, and does not suffer from substantial over-fitting, as it is still competitive when the data come from a single Student-t process rather than a mixture.

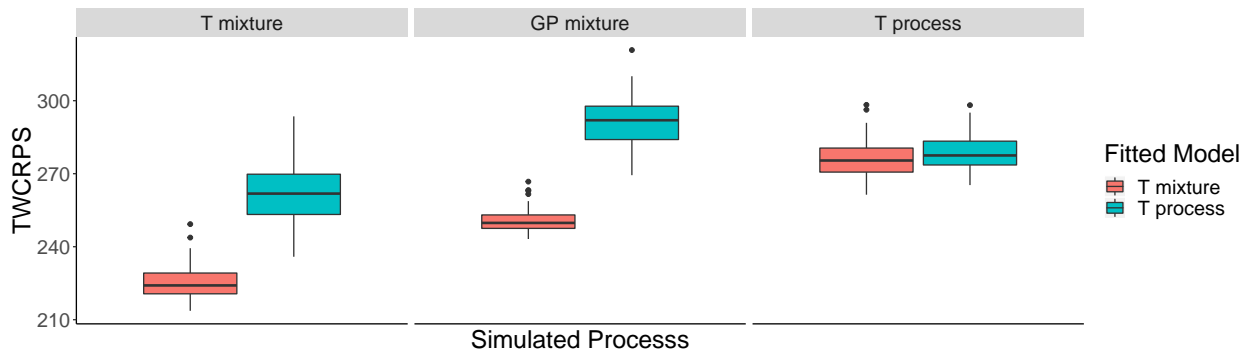

Figure 2: Tail weighted continuously ranked probability scores (TWCRPS) of total precipitation over 470 years (lower scores are better) for weight function  $w(x) = 1\{x \geq q_{0.8}\}$  where  $q_{0.8}$  is the 0.8 quantile of the simulated total precipitation data.

## References

- Gneiting, T. and M. Katzfuss (2014). Probabilistic forecasting. *Annual Review of Statistics and Its Application* 1, 125–151.
- Kay, J., C. Deser, A. Phillips, A. Mai, C. Hannay, G. Strand, J. Arblaster, S. Bates, G. Danabasoglu, J. Edwards, et al. (2015). The community earth system model (CESM) large ensemble project: A community resource for studying climate change in the presence of internal climate variability. *Bulletin of the American Meteorological Society* 96(8), 1333–1349.
